# Supplementary material for: Mpemba effect in terms of mean first passage time
Source: arXiv:2212.07496 source file (2023-05-29)
Supplement: Supplementary file 1 [file Supplementary_material_Mpemba_effect_in_terms_of_MFPT.pdf]

# Supplementary material – Mpemba effect in terms of mean first passage time


Matthew R. Walker
*Department of Physics, University of Virginia, Charlottesville, VA 22904, USA*

Marija Vucelja*
*Department of Physics, University of Virginia, Charlottesville, VA 22904, USA and*
*Department of Mathematics, University of Virginia, Charlottesville, VA 22904, USA*


## EIGENVALUE PROBLEM OF THE ADJOINT FP OPERATOR

We start with the adjoint Fokker-Planck equation and get the following eigenvalue problem

$$\mathcal{L}^\dagger u_i(x) = \frac{1}{\gamma}\left[-U'\partial_x + T_b\partial_x^2\right]u_i(x) = \frac{T_b}{\gamma}e^{\frac{U(x)}{T_b}}\partial_x e^{-\frac{U(x)}{T_b}}\partial_x u_i(x) = \lambda_i u_i(x), \tag{1}$$

which we can write as

$$\partial_x e^{-\frac{U(x)}{T_b}}\partial_x u_i(x) = \frac{\gamma\lambda_i}{T_b}e^{-\frac{U(x)}{T_b}}u_i(x). \tag{2}$$

## APPROXIMATIONS TO EXPONENTIAL INTEGRALS

In the small-diffusion limit the exponential integrals in $Z(T_b)$, $\tau_R(x_{\max})$ and $\tau_L(x_{\min})$ are readily approximated by Laplace method, leading to

$$Z(T_b) \approx \sqrt{\frac{2\pi T_b}{|U''(x_L)|}}e^{-\frac{U(x_L)}{T_b}} + \sqrt{\frac{2\pi T_b}{|U''(x_R)|}}e^{\frac{-U(x_R)}{T_b}}, \tag{3}$$

$$\tau_R(x_{\max}) \approx \frac{\gamma}{T_b}\frac{1}{2}\sqrt{\frac{2\pi T_b}{|U''(0)|}}e^{\frac{U(0)}{T_b}}\sqrt{\frac{2\pi T_b}{|U''(x_R)|}}e^{\frac{-U(x_R)}{T_b}}, \tag{4}$$

$$\tau_L(x_{\min}) \approx \frac{\gamma}{T_b}\frac{1}{2}\sqrt{\frac{2\pi T_b}{|U''(0)|}}e^{\frac{U(0)}{T_b}}\sqrt{\frac{2\pi T_b}{|U''(x_L)|}}e^{\frac{-U(x_L)}{T_b}}. \tag{5}$$

In this limit, the eigenvalue reduces to the sum of Kramer's rates from one well to another (c.f. [1]). Hence we have

$$\lambda_2 \approx -\frac{1}{2\pi\gamma}\left[e^{-\frac{U(0)-U(x_L)}{T_b}}\sqrt{|U''(0)||U''(x_L)|} + e^{-\frac{U(0)-U(x_R)}{T_b}}\sqrt{|U''(0)||U''(x_R)|}\right].$$

## MEAN FIRST PASSAGE TIME

In the 1D case, $\tau_R$ can be calculated explicitly, see e.g. [2]. Here we reproduce the main steps

$$\tau_R(x_0) = \int_0^\infty dt \int_{\mathcal{D}_R} e^{t\tilde{\mathcal{L}}}\delta(x-x_0)\,dx \tag{6}$$

$$= \int_0^\infty dt \int_{\mathcal{D}_R} \delta(x-x_0)e^{t\tilde{\mathcal{L}}^\dagger}1\,dx. \tag{7}$$

Thus we have

$$\tau_R(x) = \int_0^\infty e^{t\tilde{\mathcal{L}}^\dagger}1\,dt, \tag{8}$$

$$\tilde{\mathcal{L}}^\dagger\tau_R(x) = \int_0^\infty dt\tilde{\mathcal{L}}^\dagger e^{t\tilde{\mathcal{L}}^\dagger}1 = \int_0^\infty \frac{d}{dt}e^{t\tilde{\mathcal{L}}^\dagger}1\,it = -1, \tag{9}$$

where the upper limit vanishes because of the absorbing boundary condition. Thus mean first passage time fulfills the following differential equation

$$-\frac{U'}{\gamma}\partial_x\tau_R + \frac{T_b}{\gamma}\partial_x^2\tau_R = \frac{T_b}{\gamma}e^{\frac{U(x)}{T_b}}\partial_x e^{-\frac{U(x)}{T_b}}\partial_x\tau_R(x) = -1. \tag{10}$$

* mvucelja@virginia.edu

[1] H. Risken, *The Fokker-Planck Equation* (Springer, 1989).
[2] R. Zwanzig, *Nonequilibrium statistical mechanics* (Oxford University Press, New York, NY, USA, 2000).
